# Supplementary material for: Carrier-envelope-phase and helicity control of electron vortices in photodetachment
Source: arXiv:2205.08655 ancillary file (2022-05-17)
Supplement: Supplementary file 1 [file SupplementalMaterials.pdf]

# Supplemental Materials

*to the paper "Carrier-envelope-phase and helicity control of electron vortices in photodetachment"*
*by M. M. Majczak, F. Cajiao Vélez, J. Z. Kamiński, and K. Krajewska*

We analyze the electron photodetachment of the $H^-$ ion driven by a pair of circularly-polarized laser pulses. Each pair is considered to be in the $(\chi_1, \sigma_1; \chi_2, \sigma_2)$ configuration, where $\chi_i$ $(i = 1, 2)$ is the carrier envelope phase (CEP) of an individual pulse and $\sigma_i$ its helicity (direction of rotation). While the corotating configuration is obtained by setting $\sigma_1 = \sigma_2 \equiv \sigma$, the counterrotating case corresponds to $\sigma_1 = -\sigma_2 \equiv \sigma$. For numerical illustrations presented here, we set the peak intensity, wavelength, and number of cycles within each pulse fixed ($I = 2.5 \times 10^{11}\mathrm{W/cm}^2$, $\lambda = 4000$ nm, and $N_{\mathrm{osc}} = 3$, respectively), whereas we allow the CEPs and helicities to vary [see, Eqs. (11) to (13) in the main article].

## PHOTODEATCHMENT DRIVEN BY TWO COROTATING LASER PULSES

In this Section, we present the probability amplitude of photodetachment $\mathcal{A}(\boldsymbol{p})$ [Eqs. (5) to (7) in the main article] as a function of the electron's momentum in the $p_xp_y$-plane (i.e., we set $p_z = 0$) when a driving laser field consists of two corotating pulses. Animations 1 and 2 show the modulus (raised to the power $\nu = 0.5$, for visual purposes) and phase of the probability amplitude $\mathcal{A}(\boldsymbol{p})$, respectively. The laser field is in the configuration $(\pi/3, +; \chi, +)$, such that the CEP of the first pulse is fixed, whereas the CEP of the second pulse varies from 0 to $2\pi \approx 6.28$ rad. From both Animations we see the formation and annihilation of vortices while increasing $\chi$, together with a cyclic propagation of nodal rings towards larger momenta. Note that for $\chi = \pi/3$ we recover the probability amplitude shown in Case V (middle column of Fig. 2 in the main article).

## PHOTODEATCHMENT DRIVEN BY TWO COUNTERROTATING LASER PULSES

Similarly to the previous Section, we present here the probability amplitude of photodetachment $\mathcal{A}(\boldsymbol{p})$ in the $p_xp_y$-plane, but this time the laser field comprises two counterrotating pulses. Animations 3 and 4 show the modulus and phase of the probability amplitude $\mathcal{A}(\boldsymbol{p})$, respectively, for a driving field in the configuration $(\chi, +; \chi, -)$, i.e., both pulses have a common CEP $\chi$, which changes from 0 to $\pi$. For $\chi = 0$ and $\chi = \pi$ we observe the formation of spirals without the presence of vortex structures. Both spirals are rotated by an angle $\pi$ from one another. For any other value of the $\chi$, helical structures and vortex-antivortex pairs are observed. In particular, while increasing the CEP, a process of vortex-antivortex pair formation and annihilation is observed.

In Animations 5 and 6 we show the same as in Animations 3 and 4, respectively, but for a driving field in the configuration $(\pi/3, +; \chi, -)$, i.e., the CEP of the first pulse is $\pi/3$ while the CEP of the second pulse, $\chi$, varies from 0 to $2\pi$. This time we observe a momentum spiral which rotates clockwise while increasing $\chi$, and the appearance and mutual annihilation of vortex-antivortex pairs. At the CEP $\chi = 5\pi/3 \approx 5.2$ rad there are only nodal structures in the probability distribution of photodetachment, and no vortices are present. This is directly related to the time-reversal symmetry of the pulses, as discused in Sec. IV of the main article.

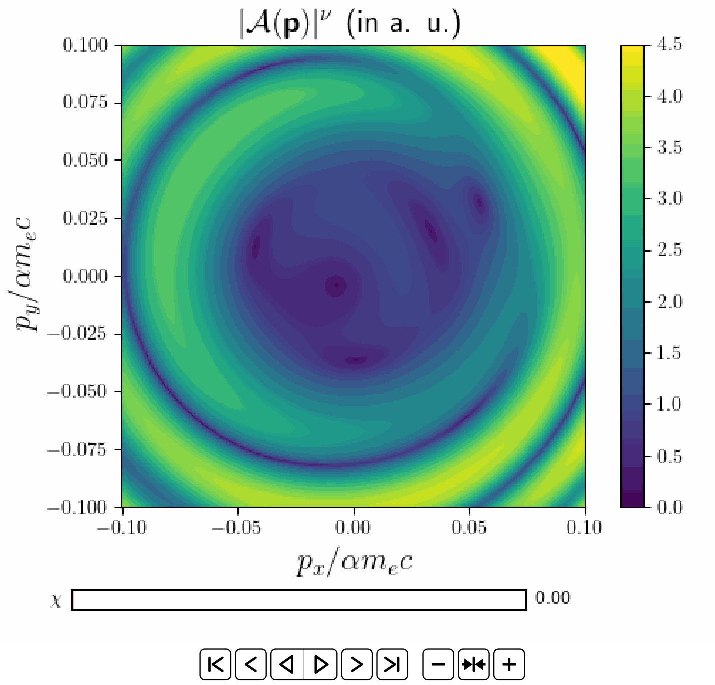


Animation 1: Modulus of the probability amplitude of detachment $|\mathcal{A}(\boldsymbol{p})|^\nu$, where $\nu = 0.5$, calculated in the $p_xp_y$-plane. The driving field consists of two corotating and circularly-polarized laser pulses in the configuration $(\pi/3, +; \chi, +)$. The peak intensity, wavelength, and number of field oscillations of the laser field are $I = 2.5 \times 10^{11}\mathrm{W/cm}^2$, $\lambda = 4000$ nm, and $N_{\rm osc} = 3$, respectively. In this Animation, the CEP changes from 0 to $2\pi$ (shown in radians) and 100 frames are used to create it.

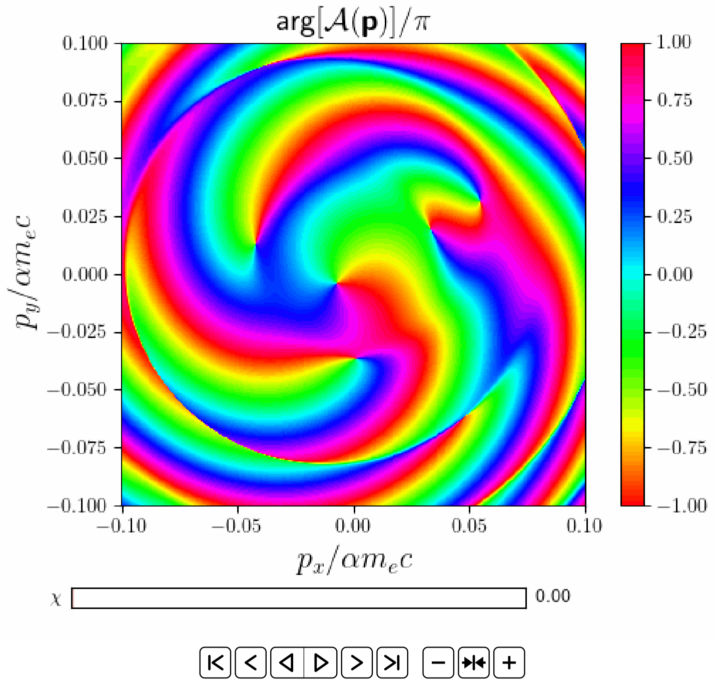


Animation 2: Phase of the probability amplitude of detachment $\arg[\mathcal{A}(\boldsymbol{p})]/\pi$, corresponding to Fig. 1. Again, 100 frames were used to create this Animation.

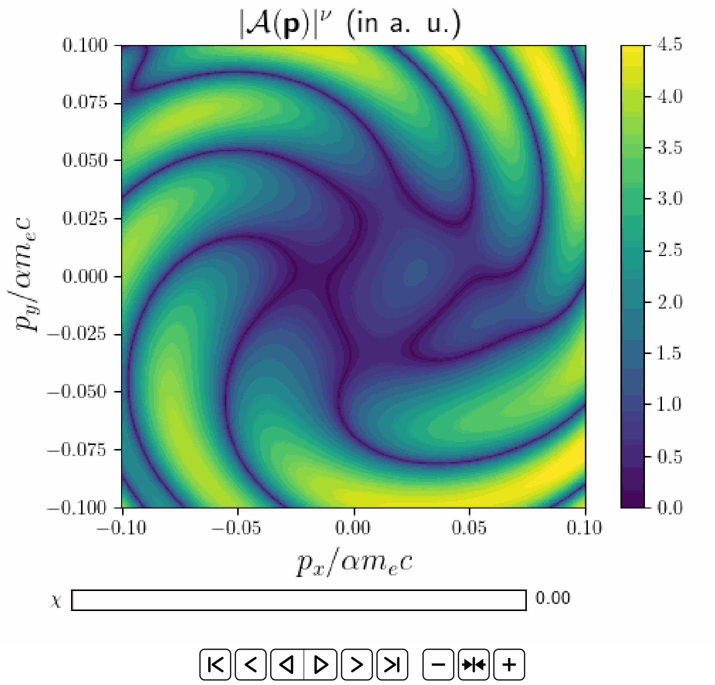


Animation 3: The same as in Animation 1 but for a driving field consisting of a sequence of two counterrotating and circularly-polarized pules. The train of pulses is in the configuration $(\chi, +; \chi, -)$ and $\chi$ varies from 0 to $\pi$.

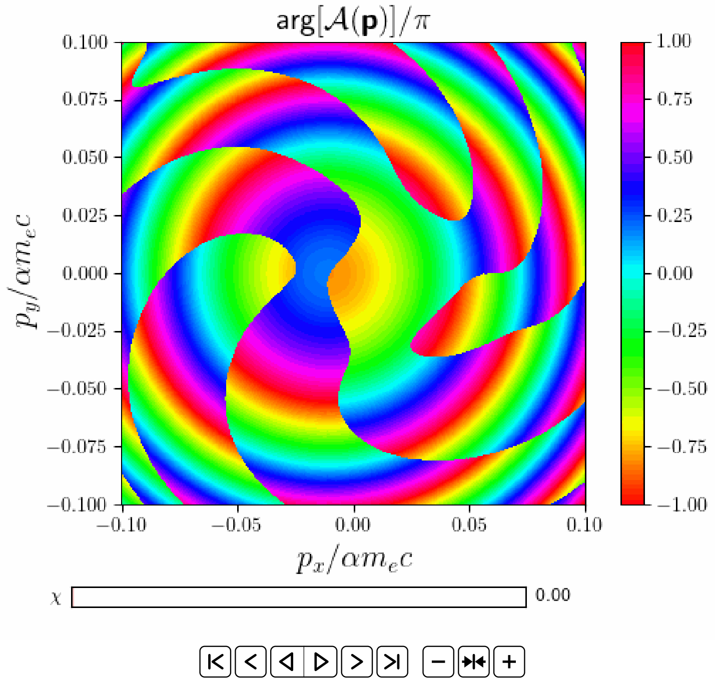


Animation 4: The same as in Animation 2 but for a driving field in the configuration $(\chi, +; \chi, -)$, where $\chi$ varies from 0 to $\pi$.

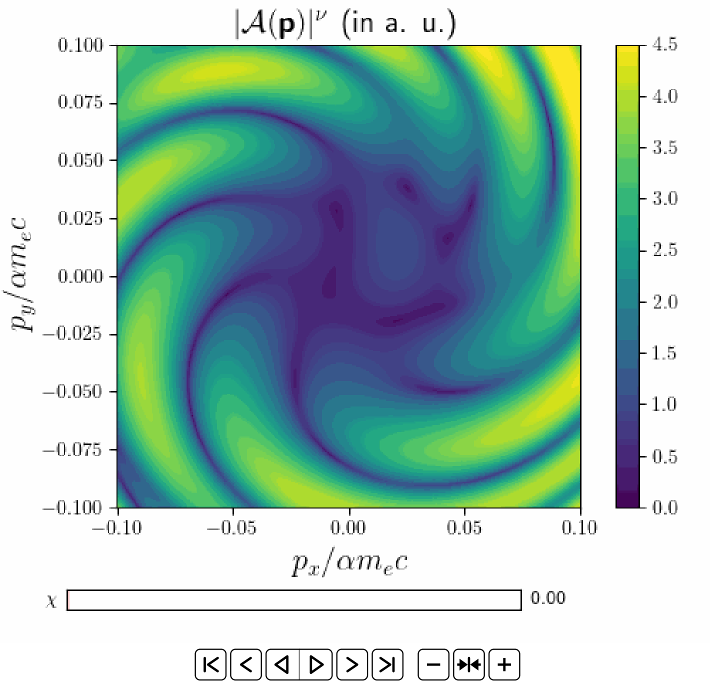


Animation 5: The same as in Animation 3 but for a driving field in the configuration $(\pi/3, +; \chi, -)$: while the CEP of the first pulse is set to $\pi/3$, the CEP of the second pulse varies from 0 to $2\pi$.

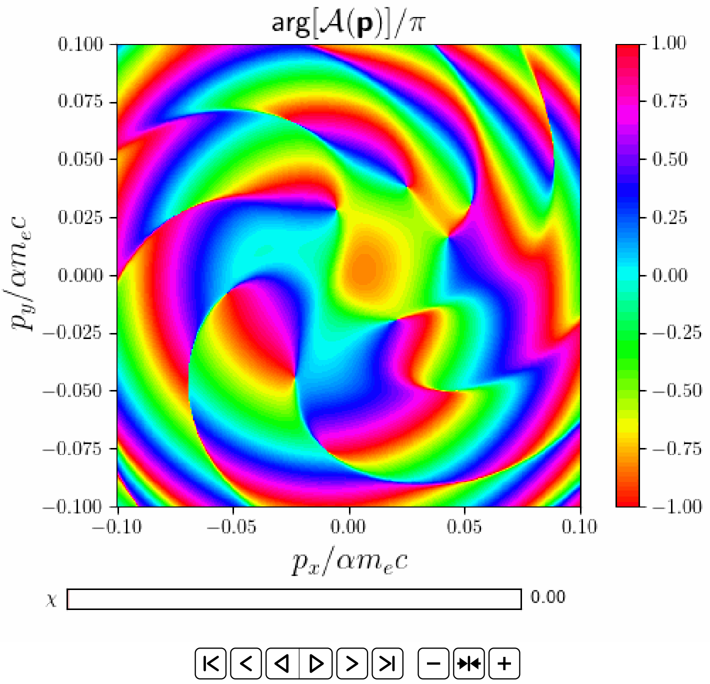


Animation 6: The same as in Animation 4 but for a driving field in the configuration $(\pi/3, +; \chi, -)$, and the CEP varying from 0 to $2\pi$.
